# Supplementary material for: AURA: Amplifying Understanding, Resilience, and Awareness for Responsible AI Content Work
Source: arXiv:2411.01426 source file (2024-11-03)
Supplement: Supplementary file 1 [file 9_appendix.tex]

% \section{Supplementary Materials}
% In the following section, we include additional materials, including \edit{survey questions, interview questions, frequently asked questions shared during recruitment,} graphics shown during our workshops\edit{,} and snapshots of our workshop information. 

% \subsection{Survey questions}\label{appendix:survey}
% Questions 1-2 asked for participant consent and for participants to complete a captcha.\\
% \subsubsection{Tell us about yourself}

% \textbf{Q3.2 What is your age?}
% \begin{itemize}
%     \item 18-25 years old
%     \item 26-35 years old
%     \item 36-45 years old
%     \item 46-55 years old
%     \item 56-65 years old
%     \item 66+ years old
%     \item Prefer not to say
% \end{itemize}\\

% \textbf{Q3.3 How do you describe your gender identity?}
% \begin{itemize}
%     \item Female/Women (some examples: cisgender women, female-identified people, transgender women)
%     \item Gender nonbinary (some examples: gender diverse, gender fluid, gender non-conforming, gender questioning, genderqueer, nonbinary, two-spirit)
%     \item Transgender (some examples: transgender female, transgender male, transgender non-conforming, nonbinary)
%     \item Male/Men (some examples: cisgender men, male-identified people, transgender men)
%     \item Unsure
%     \item Not listed or prefer to self-describe
%     \item Prefer not to say
% \end{itemize}

% \textbf{Q3.4 What is the highest level of education you have achieved?}
% \begin{itemize}
%     \item Less than high school
%     \item High school diploma or equivalent
%     \item Some college or vocational training
%     \item Bachelor's degree
%     \item Some postgraduate degree
%     \item Master's degree
%     \item Doctoral or professional degree
%     \item Prefer not to say
% \end{itemize}

% \textbf{Q3.5 What is your employment status?}
% \begin{itemize}
%     \item Full-time employee
%     \item Part-time employee
%     \item Full-time contractor
%     \item Part-time contractor
%     \item Volunteer
%     \item Other
% \end{itemize}

% \textbf{Q3.6 Which of the following activities do you perform as part of your job? Please select all that apply.}
% \begin{itemize}
%     \item Content Moderation: I review various forms of online content (including text, photos, audio, and video) with the intent to flag or identify any content that potentially violates the platform's policy or guidelines. This could lead to the content's modification or removal to ensure the platform maintains a safe and respectful environment.
%     \item Data Labeling: My work primarily involves reviewing, labeling, or categorizing various types of content (including text, photos, audio, and video). This is done according to specific labeling or sorting guidelines, which aids in data analysis and training machine learning models.
%     \item Red-Teaming: I conduct critical assessments of product or platform features by simulating the actions of potential bad actors or testing system vulnerabilities. The objective is to identify if these features can inadvertently generate or promote content that violates policy or guidelines, thus enhancing the product's security and safety measures.
% \end{itemize}

% \textbf{Q3.7 How would you describe your involvement in content moderation?}
% \begin{itemize}
%     \item It is my primary job responsibility.
%     \item It is part of my job responsibilities, but not the main focus.
%     \item I volunteer or participate in my free time.
%     \item Other (please specify)
% \end{itemize}

% \textbf{Q3.8 How would you describe your involvement in data labeling?}
% \begin{itemize}
%     \item It is my primary job responsibility.
%     \item It is part of my job responsibilities, but not the main focus.
%     \item I volunteer or participate in my free time.
%     \item Other (please specify)
% \end{itemize}

% \textbf{Q3.9 How would you describe your involvement in the Red Team?}
% \begin{itemize}
%     \item It is my primary job responsibility.
%     \item It is part of my job responsibilities, but not the main focus.
%     \item I volunteer or participate in my free time.
%     \item Other (please specify)
% \end{itemize}


% \textbf{Q3.10 How long have you been working as a content moderator? (Please sum up all the months and years of experience as a content moderator, even if there were breaks in between.)}
% \begin{itemize}
%     \item Less than 6 months
%     \item 6 months to 1 year
%     \item 1 to 2 years
%     \item 2 to 5 years
%     \item More than 5 years
%     \item Prefer not to say
% \end{itemize}


% \textbf{Q3.11 How long have you been working as a data labeler? (Please sum up all the months and years of experience as a data labeler, even if there were breaks in between.)}
% \begin{itemize}
%     \item Less than 6 months
%     \item 6 months to 1 year
%     \item 1 to 2 years
%     \item 2 to 5 years
%     \item More than 5 years
%     \item Prefer not to say
% \end{itemize}

% \textbf{Q3.12 How long have you been working in the Red Team? (Please sum up all the months and years of experience in the Red Team, even if there were breaks in between.)}
% \begin{itemize}
%     \item Less than 6 months
%     \item 6 months to 1 year
%     \item 1 to 2 years
%     \item 2 to 5 years
%     \item More than 5 years
%     \item Prefer not to say
% \end{itemize}

% \textbf{Q3.13 What motivated you to take on the role of a content moderator, a data labeler, or a red team member? (Please do not include any information in your response that could be used to identify you as an individual or your employer.)}

% \textbf{Q4.1 Please tell us about the work you do. For the following questions, when we refer to reviewing content, we mean all content that is either generated (by you or by product/platform features) or reviewed (by you) as part of your content moderation, data labeling, or red-teaming activities.}

% \textbf{Q4.2 What type of content do you review? (Select all that apply)}
% \begin{itemize}
%     \item Text
%     \item Images
%     \item Videos
%     \item Audio
%     \item Live streams
%     \item Other
% \end{itemize}

% \textbf{Q4.3 On average, how many hours do you spend reviewing content per week?}
% \begin{itemize}
%     \item Less than 10 hours
%     \item 10 to 20 hours
%     \item 20 to 30 hours
%     \item 30 to 40 hours
%     \item More than 40 hours
% \end{itemize}

% \textbf{Q4.4 On average, how many contiguous hours do you spend reviewing content per day?}
% \begin{itemize}
%     \item Less than 1 hour
%     \item 1 to 2 hours
%     \item 2 to 3 hours
%     \item 3 to 4 hours
%     \item More than 4 hours
% \end{itemize}

% \textbf{Q4.5 What categories of content do you review? Please select all that apply.}
% \begin{itemize}
%     \item Child abuse or exploitation: Depictions of child abuse, child pornography, or any content that exploits or endangers minors.
%     \item Terrorism and extremist content: Content promoting or supporting terrorism, violent extremism, or the recruitment of individuals for such activities.
%     \item Hate speech and acts: Language, imagery, or actions that promote hatred, discrimination, or violence against individuals or groups based on factors such as race, ethnicity, religion, gender, sexual orientation, or disability.
%     \item Harassment and bullying: Content that targets, harasses, or bullies individuals, including personal attacks, defamation, or intimidation.
%     \item Graphic violence and gore: Depictions of excessive violence, injuries, or gore, including real-life acts of violence or cruelty, as well as fictional representations in movies, games, or other media.
%     \item Self-harm and suicide: Content that promotes, encourages, or glorifies self-harm, suicide, or other harmful behaviors.
%     \item Sexual content and nudity: Explicit sexual content, pornography, or non-consensual sharing of intimate images or videos (revenge porn), as well as gratuitous nudity or sexually suggestive material.
%     \item Illegal activities: Content that promotes, encourages, or provides information about illegal activities, such as drug use, theft, or hacking.
%     \item Misinformation and disinformation: False, misleading, or deceptive information, including conspiracy theories, deepfake videos, or manipulated content.
%     \item Copyright infringement: Content that violates intellectual property rights, such as sharing copyrighted music, movies, or images without proper authorization.
%     \item Spam and scams: Content that is intended to deceive, manipulate, or exploit users, including phishing, malware, or other fraudulent schemes, as well as spam or unsolicited promotional material.
%     \item Privacy violations: Content that invades the privacy of individuals, such as sharing personal information without consent, stalking, or doxing.
%     \item Impersonation: Content that falsely represents a person or entity, including fake accounts, profiles, or pages created to deceive or mislead others.
%     \item Other
% \end{itemize}


% \textbf{Q4.6 How would you rate the overall quality of your sleep since you started working as a content moderator, a data labeler, or a red-team member?}
% \begin{itemize}
%     \item Very poor - I consistently have difficulty falling asleep, staying asleep, or experience restless and non-restorative sleep.
%     \item Poor - I frequently have difficulty falling asleep, staying asleep, or experience restless and non-restorative sleep, but there are occasional nights with better sleep quality.
%     \item Fair - I have a mix of good and bad nights, with some difficulty falling asleep, staying asleep, or experiencing restless and non-restorative sleep.
%     \item Good - I generally sleep well, with only occasional difficulties falling asleep, staying asleep, or experiencing restless and non-restorative sleep.
%     \item Very good - I consistently sleep well, with minimal to no difficulties falling asleep, staying asleep, or experiencing restless and non-restorative sleep.
% \end{itemize}

% \textbf{Q4.7 Have you ever experienced nightmares, flashbacks, or intrusive thoughts related to the content you review?}
% \begin{itemize}
%     \item Never
%     \item Extremely rarely - less than once a year
%     \item Very rarely - less than once per month
%     \item Rarely - less than once per week
%     \item Occasionally - Once to twice per week
%     \item Frequently - 3 to 5 times per week
%     \item Almost always - 6 or more times per week
% \end{itemize}

% \textbf{Q4.8 Has your work as a content moderator, a data labeler, or a red-team member impacted you positively? If so, please describe how. (Please do not include any information in your response that could be used to identify you as an individual or your employer.)}

% \textbf{Q4.9 Has your work as a content moderator, a data labeler, or a red-team member impacted you negatively? If so, please describe how. (Please do not include any information in your response that could be used to identify you as an individual or your employer.)}

% \textbf{Q4.10 Has your work as a content moderator, a data labeler, or a red-team member been impacted by the recent rise in the use of generative AI technologies (e.g., large language models like OpenAI ChatGPT, image generation models like DALL-E)? If so, please describe how. (Please do not include any information in your response that could be used to identify you as an individual or your employer.)}

% \textbf{Q5.1 Please tell us about challenges of your work and opportunities for supporting your work.}

% \textbf{Q5.2 In your opinion, what are the most significant challenges facing content moderators, data labelers, and red-team members today? (Please do not include any information in your response that could be used to identify you as an individual or your employer.)}

% \textbf{Q5.3 What are some ways that the challenges that you outlined above can or should be addressed by technology? (Please do not include any information in your response that could be used to identify you as an individual or your employer.)}

% \textbf{Q5.4 If you could change one aspect of your role as a content moderator, a data labeler, and a red-team member, what would it be and why? (Please do not include any information in your response that could be used to identify you as an individual or your employer.)}

% \textbf{Q6.1 The following question is to verify that you are a real person. Please select ‘disagree’ to this question.}
% \begin{itemize}
%     \item Strongly disagree
%     \item Disagree
%     \item Neutral
%     \item Agree
%     \item Strongly agree
% \end{itemize}

% \textbf{Q7.1 Please tell us about the tools that you use for work.}

% For the following questions, when we refer to reviewing content, we mean all content that is either generated (by you or by product/platform features) or reviewed (by you) as part of your content moderation, data labeling, or red-teaming activities.

% \textbf{Q7.2 For each of the tools below, please indicate their usefulness while reviewing content, both directly (i.e., it helps me review the content more accurately or efficiently) or indirectly (i.e., it helps me reduce potentially negative impacts associated with reviewing upsetting content).}

% \textbf{Scale:}
% \begin{itemize}
%     \item I don't have access to this
%     \item I never used this
%     \item Not at all useful
%     \item Slightly useful
%     \item Moderately useful
%     \item Very useful
%     \item Extremely useful
% \end{itemize}

% \textbf{Tools:}
% \begin{itemize}
%     \item Automated verification or vetting of user accounts
%     \item Automated warning about certain contents as potentially triggering
%     \item Automated content summarization
%     \item Automated content labeling
%     \item Automated assistance on bringing relevant guideline information for content moderation
%     \item Automated assistance on viewing similar or example content for comparison and decision-making
%     \item Applying monochrome, grey scale, or color filter on visual content
%     \item Blurring of visual content (e.g., blurring face)
%     \item Blocking of visual content (e.g., blocking face)
%     \item Turning off audio and viewing the video only
%     \item Reducing audio volume
%     \item Increasing audio volume
%     \item Turning off video and listening to audio only
%     \item Reducing the speed of audio or video
%     \item Increasing the speed of audio or video
%     \item Listening to other music while viewing the video or text only
%     \item Having control over what part of the content is seen or heard
%     \item Having control over how the content is seen or heard
% \end{itemize}

% \textbf{Q7.3 If there are tools that you found useful while reviewing content which are not mentioned above, please describe them here. (Please do not include any information in your response that could be used to identify you as an individual or your employer.)}

% \textbf{Q8.1 Please tell us about how you manage demands from work.}

% For the following questions, when we refer to reviewing content, we mean all content that is either generated (by you or by product/platform features) or reviewed (by you) as part of your content moderation, data labeling, or red-teaming activities.

% \textbf{Q8.2 For each of the activities below, please indicate their usefulness for managing the demands of reviewing content and its impact on your overall wellbeing (e.g., positive coping after viewing upsetting content).}

% \textbf{Scale:}
% \begin{itemize}
%     \item I don't have access to this
%     \item I never used this
%     \item Not at all useful
%     \item Slightly useful
%     \item Moderately useful
%     \item Very useful
%     \item Extremely useful
% \end{itemize}

% \textbf{Activities:}
% \begin{itemize}
%     \item Changing my work environment (e.g., lighting, temperature)
%     \item Listening to music
%     \item Taking breaks from content moderation
%     \item Conducting distracting activities between content moderation
%     \item Being creative
%     \item Playing games (e.g., video games, board games)
%     \item Tracking and monitoring my physical and mental health throughout the day, week, or month
%     \item Using wearables (e.g., Fitbit, Apple Watch, Oura) to track health, sleep, or mood
%     \item Engaging in relaxation or spiritual practices (e.g., mindfulness, meditation, deep breathing, praying)
%     \item Practicing gratitude, positive thinking, reframing negative thoughts
%     \item Journaling, expressive writing, or reflecting on the day
%     \item Disconnecting from work and/or devices
%     \item Being in nature or outside
%     \item Moving your body (e.g., exercising, walking, stretching)
%     \item Socializing or chatting with colleagues
%     \item Being alone or having a quiet moment alone
%     \item Taking care of basic needs (e.g., eating, hydrating)
%     \item Resting, napping, or sleeping
%     \item Drinking alcoholic beverages or using recreational substances
%     \item Engaging in fun or entertaining activities (e.g., reading, watching TV, shopping)
%     \item Daydreaming
%     \item Getting emotional support from others (e.g., friends, family)
%     \item Seeing a professional therapist or a counselor
%     \item Taking resilience or wellness training or classes
%     \item Planning, task management, or problem-solving
% \end{itemize}

% \textbf{Q8.3 If there are tools that you found useful for managing the demands of reviewing content and its impact on your overall wellbeing which are not mentioned above, please describe them here. (Please do not include any information in your response that could be used to identify you as an individual or your employer.)}


% \textbf{Q8.4 Based on your experience with any of the tools used during content review and for managing the demands of reviewing content and its impact on your overall wellbeing, what are some high priority challenges with the tools that should be addressed? (Please do not include any information in your response that could be used to identify you as an individual or your employer.)}

% \textbf{Q8.5 What other comments or suggestions related to content moderation, data labeling, or red-teaming, its challenges, or potential improvements in the field do you have? (Please do not include any information in your response that could be used to identify you as an individual or your employer.)}


% \textbf{Q9.1 Please try to form the images described below and rate each mental image on the following scale: 0 (no image at all) to 10 (image as clear and vivid as real life).}

% \textbf{Q9.2 Imagine the appearance of:}

% \begin{itemize}
%     \item a cat climbing a tree
%     \item a sunset
%     \item a bonfire
% \end{itemize}

% \textbf{Q9.3 Imagine the sound of:}

% \begin{itemize}
%     \item a car horn
%     \item hands clapping in applause
%     \item an ambulance siren
% \end{itemize}

% \textbf{Q9.4 Imagine the smell of:}

% \begin{itemize}
%     \item a rose
%     \item newly cut grass
%     \item burning wood
% \end{itemize}

% \textbf{Q9.5 Imagine the taste of:}

% \begin{itemize}
%     \item mustard
%     \item lemon
%     \item black pepper
% \end{itemize}

% \textbf{Q9.6 Imagine touching:}

% \begin{itemize}
%     \item warm sand
%     \item a soft towel
%     \item fur
% \end{itemize}

% \textbf{Q9.7 Imagine the bodily sensation of:}

% \begin{itemize}
%     \item relaxing in a warm bath
%     \item jumping into a swimming pool
%     \item walking briskly in the cold
% \end{itemize}

% \textbf{Q9.8 Imagine feeling:}

% \begin{itemize}
%     \item excited
%     \item relieved
%     \item scared
% \end{itemize}


% \textbf{Q10.1 The following statements are related to your work situation and how you experience this situation. Please state how often each statement applies to you.}

% \textbf{Scale:}
% \begin{itemize}
%     \item Never
%     \item Rarely
%     \item Sometimes
%     \item Often
%     \item Always
% \end{itemize}

% \textbf{Statements:}
% \begin{itemize}
%     \item At work, I feel mentally exhausted
%     \item Everything I do at work requires a great deal of effort
%     \item After a day at work, I find it hard to recover my energy
%     \item At work, I feel physically exhausted
%     \item When I get up in the morning, I lack the energy to start a new day at work
%     \item I want to be active at work, but somehow, I am unable to manage
%     \item When I exert myself at work, I quickly get tired
%     \item At the end of my working day, I feel mentally exhausted and drained
%     \item I struggle to find any enthusiasm for my work
%     \item At work, I do not think much about what I am doing and I function on autopilot
%     \item I feel a strong aversion towards my job
%     \item I feel indifferent about my job
%     \item I'm cynical about what my work means to others
%     \item At work, I have trouble staying focused
%     \item At work I struggle to think clearly
%     \item I'm forgetful and distracted at work
%     \item When I'm working, I have trouble concentrating
%     \item I make mistakes in my work because I have my mind on other things
%     \item At work, I feel unable to control my emotions
%     \item I do not recognize myself in the way I react emotionally at work
%     \item During my work I become irritable when things don't go my way
%     \item I get upset or sad at work without knowing why
%     \item At work I may overreact unintentionally
%     \item I have trouble falling or staying asleep
%     \item I tend to worry
%     \item I feel tense and stressed
%     \item I feel anxious and/or suffer from panic attacks
%     \item Noise and crowds disturb me
%     \item I suffer from palpitations or chest pain
%     \item I suffer from stomach and/or intestinal complaints
%     \item I suffer from headaches
%     \item I suffer from muscle pain, for example in the neck, shoulder or back
%     \item I often get sick
% \end{itemize}

% \textbf{Q11.1 We would like to ask you some questions about your emotional life, in particular, how you control (that is, regulate and manage) your emotions. The questions below involve two distinct aspects of your emotional life. One is your emotional experience, or what you feel like inside. The other is your emotional expression, or how you show your emotions in the way you talk, gesture, or behave. Although some of the following questions may seem similar to one another, they differ in important ways. For each item, please answer using the following scale:}

% \begin{itemize}
%     \item Strongly disagree
%     \item Disagree
%     \item Somewhat disagree
%     \item Neither agree or disagree
%     \item Somewhat agree
%     \item Agree
%     \item Strongly agree
% \end{itemize}

% \textbf{Statements:}
% \begin{itemize}
%     \item When I want to feel more positive emotion (such as joy or amusement), I change what I’m thinking about.
%     \item I keep my emotions to myself.
%     \item When I want to feel less negative emotion (such as sadness or anger), I change what I’m thinking about.
%     \item When I am feeling positive emotions, I am careful not to express them.
%     \item When I’m faced with a stressful situation, I make myself think about it in a way that helps me stay calm.
%     \item I control my emotions by not expressing them.
%     \item When I want to feel more positive emotion, I change the way I’m thinking about the situation.
%     \item I control my emotions by changing the way I think about the situation I’m in.
%     \item When I am feeling negative emotions, I make sure not to express them.
%     \item When I want to feel less negative emotion, I change the way I’m thinking about the situation.
% \end{itemize}

% \textbf{Q12.1 Compensation and Follow-up}

% \textbf{Q12.2 Thank you for participating in the survey to help us explore innovative ways to support content moderators, data labelers, and red-team members. Before we let you go, would you like to receive a gift card for your time spent providing your survey responses? Your survey response will still remain anonymous.}

% \begin{itemize}
%     \item Yes, I would like to receive a gift card.
%     \item No, I do not want a gift card.
% \end{itemize}

% \textbf{Q12.3 We are looking for participants to join a follow-up interview study to share more insights about their experiences or to envision technology support for content moderators, data labelers, and red-team members. The interview will be conducted online and will take about 1 hour. You will receive a \$50 gift card as a token of appreciation. Would you like to be contacted with the follow-up study information? Your survey response will still remain anonymous.}

% \begin{itemize}
%     \item Yes, please contact me with follow-up study information.
%     \item No, I am not interested in a follow-up study at this time.
% \end{itemize}


% \subsection{Interview questions}\label{appendix:interview}
% The following protocol contains questions we asked during our semi-structured interviews. We structured interview questions into four main sections to examine the aspects of the nature of content work outlined in RQ1. Keeping the semi-structured nature of the interview in mind, the questions we present below include a superset of questions that could asked during the interview based on the discussion. If screen sharing was involved, we specifically requested our participants not to share any potentially harmful or sensitive content with the researchers.

% \subsubsection{Grounding}
% Please choose one of the following activities as your primary activity: 
% \begin{itemize}
%     \item \textbf{Content Moderation:} I review various forms of online content (including text, photos, audio, and video) with the intent to flag or identify any content that potentially violates the platform's policy or guidelines. This could lead to the content's modification or removal to ensure the platform maintains a safe and respectful environment. 
%     \item \textbf{Data Labeling:} My work primarily involves reviewing, labeling, or categorizing various types of content (including text, photos, audio, and video). This is done according to specific labeling or sorting guidelines, which aids in data analysis and training machine learning models. 
%     \item \textbf{Red-Teaming:} I conduct critical assessments of product or platform features by simulating the actions of potential bad actors or testing system vulnerabilities. The objective is to identify if these features can inadvertently generate or promote content that violates policy or guidelines, thus enhancing the product's security and safety measures. 
% \end{itemize}
% To help us understand your experience with this activity, tell us about this activity. What does it entail? Where does this work come from? What are you trying to achieve with this work? For the following questions, let’s use this specific activity that you described as your “work.”  

% \subsubsection{Work Setup}
% Could you describe your work setting, including where you work, hardware or software you work with, people you work with, your work environment? 
% \begin{itemize}
%     \item \textbf{Location:} Where are you doing the work (desk, cubicle, etc.)?
%     \item \textbf{Equipment:} What do you work with (hardware, software)?
%     \item \textbf{Environment:} What is the environment like (noise, temperature, comfort level generally)?
%     \item \textbf{People:} Who is around you (individual vs. collaborative work)?
%     \item \textbf{Ideal Setup:} What would your ideal setup (including location, environment, people) be? What are the barriers to accessing this ideal setup?
% \end{itemize}

% \subsubsection{Conducting Work}
% \begin{itemize}
%     \item What tools do you use to help you with this work? Who develops the tool?
%     \item  What support from other people is most helpful for you in your work?
%     \item How helpful are automated (AI) tools for your daily work? If you could request changes to how automated tools work, what changes would you want?
%     \item What is an ideal tool that would help with your work, what would that look like? Why? What are the barriers to accessing this ideal tool?
%     \item How have generative AI tools impacted you doing your work (either/both as a solution and problem)? 
%     \item How have generative AI tools impacted \textit{the demands} of your work (either/both as a solution and problem)? 
% \end{itemize}


% \subsubsection{Coping}
% Tell me about a time when your well-being was impacted by the content moderation/data labeling/red-teaming work you do.
% \begin{itemize}
%     \item What strategies, resources, and support were helpful for improving your well-being? (organizational vs. ad-hoc)
%     \item What other strategies, resources, and support would you want to have access to in an ideal scenario? (organizational vs. ad-hoc)
%     \item What support from other people is helpful for managing these demands (i.e., do you share tips, talk with co-workers, managers, etc. about wellness)? What are the barriers to accessing these strategies, resources, and supports?
%     \item  If you were to wave a magic wand to create any kind of technology/software/UX experience that would help with managing the demands of or coping with your work, what would that look like? Why? (e.g., help coping with stress and anxiety, or maladaptive memories) What would a tool like that look like? (e.g., VR immersive interface, or audio-only based interventions, scent and other modalities, an empathic agent, etc.)
%     \item If you were to wave a magic wand to create any kind of resource or activity that would help with managing the demands of or coping with your work, what would that look like? Why?
%     \item What resources, tools, or activities have been most helpful in managing the demands of your work (e.g., training, breaks, etc.)? Which of these resources, tools, or activities do you use at work or outside of work? How does the modality of these resources impact how helpful they are (for remote workers, is it necessary to have in-person access and vice versa)?
%     \item What other strategies do you use to cope with the demands of your work? (e.g., meditation, video games)
%     \item What other support is most helpful for managing emotional and wellbeing demands of your work?
%     \item Which of these supports (resources, strategies, support from other people) is formally provided/encouraged by your organization?
%     \item  Which of these are ad hoc?
%     \item How does the organizational and ad hoc support you have differ from your ideal amount of support?
% \end{itemize}

% \subsubsection{Collaboration}
% \begin{itemize}
%     \item How do you decide how to classify content or generate adversarial content?What do you do when you see content or behavior that is more in the “grey” area?
%     \item Who do you work with to make these decisions (co-workers vs managers)? Who needs to approve your decisions? Who supports you in these decisions?
%     \item What about this process is challenging for your work? What is most helpful?
% \end{itemize}


% \subsection{Frequently asked questions (FAQ) about the study}

% The following FAQ was shared with the potential participants during recruitment for our survey and interviews. Please note that we emphasized the anonymity of the responses to protect the identify of our participants and to minimize the risk of retaliation by the employers if identified. 


% \paragraph{What is Microsoft Research? }

% Microsoft Research is an academic arm of Microsoft. Although Microsoft Research is funded by Microsoft, the research conducted by Microsoft Research follows the same standards that academic institutions follow to conduct their research. Microsoft Research, as a research institution, not only conforms to the privacy and security regulations governed by the company but also follows the federal ethical guidelines. Additionally, Microsoft Research is able to retain academic freedom and discourse without our research topics requiring approval by PR or marketing. 

 
% \paragraph{Why are you conducting this study? }

% We are interested in understanding the perspectives and experiences of content moderators, data labelers, and red-team members who deal with various types of online content on a daily basis. The purpose of this research is to develop an understanding of the nature of content moderation, data labeling, and red-teaming work and the tools being used that directly and indirectly impact the work. We hope to identify the challenges and opportunities for improving and supporting the work of content moderators, data labelers, and red-team members.   

 

% \paragraph{Who can participate in this study? }

% We are looking for participants that conduct content or feature review tasks as part of their job. As part of your job, you may be exposed to potentially disturbing or impactful content. A content moderator is someone who reviews online content (text, photo, audio, video) to determine its suitability for a platform or a product based on its policy or guidelines. A data labeler reviews, labels, and categorizes various types of content according to specific labeling or sorting guidelines, which aids in data analysis or training machine learning models. A red-team member conducts critical assessments of product or platform features by simulating the actions of potential bad actors or testing system vulnerabilities. While you do not need to be doing these tasks full-time, you need to spend at least 1 hours/week reviewing content or features and have been working as a content moderator, a data labeler, or a red-team member for at least 3 months to be eligible. You must also be at least 18 years old. 


% \paragraph{Will my employer know that I’m participating? }

% The survey does not ask for or collect any information about your employer. Participating in this study will not affect your employment. Any information we collect about you and as part of study coordination will not be linked to your responses and will not be shared with your employer. 

 

% \paragraph{How will you use the data from the study? }

% We will use the data to analyze the themes and patterns that emerge from the responses. We will also use the data to generate recommendations and suggestions for improving and supporting content moderation, data labeling, or red-teaming work. We will publish our findings in academic journals and conferences, as well as share them with relevant stakeholders and organizations. 

 

% \paragraph{How will you protect my privacy and confidentiality? }

% The survey is anonymous. We will only collect your name and email address for the purpose of sending you your gift card and information about follow-up interviews, both of which are optional.   

% \subsection{Workshop Materials}
% The workshops were structured into three main segments:

% \begin{enumerate}
%     \item \textit{Orientation (10 minutes):} We first gave a quick tutorial on FigJam and asked everyone to introduce themselves. We used this as an exercise to post sticky notes and to react to each other's notes using stamps.
%     \item \textit{Validating discovered challenges (20 minutes):} We shared 11 challenge cards~(\autoref{fig:challenge_and_recommendation_cards} left), each describing one challenge theme discovered in phase 1 and a set of example quotes that illustrate that challenge theme. The example quotes were generated by interpreting and paraphrasing qualitative data from the first phase to preserve anonymity and to evaluate our interpretation. We asked participants to independently look through each challenge card, and vote on those that they agree or disagree with, comment on whether they think the challenge is accurate, and react to each other's notes. If there were missing challenges, they were asked to generate a new challenge card. We finished with a quick discussion of emerging themes. A zoomed-in screenshot of the challenge board is shown in \autoref{fig:challenges_zoom}.
%     \item \textit{Reviewing recommendations (30 minutes): } We introduced the AURA framework with its preliminary recommendations from phase 1. Each recommendation card~(\autoref{fig:challenge_and_recommendation_cards} right) stated the recommendation and an example of how that recommendation could be implemented. We asked participants to independently review each recommendation card and comment on what they liked, what they didn't like, what they would change, and how they would want the recommendation implemented. Just as before, they can read and react to each other's notes and can add new recommendation cards if any are missing. As a group, we discussed emerging themes, how the recommendations could be improved, and how our recommendations may be implemented. A zoomed-in screenshot of the recommendation board is shown in \autoref{fig:recommendations_zoom}.
% \end{enumerate}

% The workshop sessions had slight variations from each other because of the makeup of the group and the comfort level of participants to speak up. The facilitator generally asked for volunteers to speak up or called out participants to elaborate on their stickies to encourage active participation from everyone in the session.

% \begin{figure}[!h]
%   \centering
%   \includegraphics[width=\textwidth]{Images/challenge_and_recommendation_cards.png}
%   \caption{A full set of challenge (left) and recommendation (right) cards used in our workshops. }
%   \label{fig:challenge_and_recommendation_cards}
% \end{figure}


% \begin{figure}
%     \centering
%     \includegraphics[width=\textwidth]{Images/workshop_challenge.pdf}
%     \caption{A zoomed-in snapshot of the discussion of challenges in our workshop. For each challenge, we asked participants to write about their agreements and examples of what the challenge might look like. Participants reacted to each other's stickies. Participants additionally added thumbs-up stickers for challenges they agreed with the most across all challenges.}
%     \label{fig:challenges_zoom}
% \end{figure}
% % \footnotetext[4]{Details are anonymized for participant privacy}

% \begin{figure}
%     \centering
%     \includegraphics[width=\textwidth]{Images/workshop_recommendation.pdf}
%     \caption{A zoomed-in snapshot of the discussion of our recommendations. For each recommendation, we asked participants to write about their likes, dislikes, and examples of what the recommendation might look like. Participants reacted to each other's stickies. }
%     \label{fig:recommendations_zoom}
% \end{figure}
